# Supplementary material for: Another Vertical View: A Hierarchical Network for Heterogeneous Trajectory Prediction via Spectrums
Source: arXiv:2304.05106 source file (2024-12-03)
Supplement: Supplementary file 1 [file s4_AGraphView.tex]

%%%%%%%%%%%%%%%%%%%%%%%
%% Author: Conghao Wong
%% Date: 2023-04-18 20:27:26
%% LastEditors: Beihao Xia
%% LastEditTime: 2023-06-26 19:57:46
%% Description: file content
%% Github: https://cocoon2wong.github.io
%% Copyright 2023 Conghao Wong, All Rights Reserved.
%%%%%%%%%%%%%%%%%%%%%%%

\documentclass[../../paper.tex]{subfiles}

\begin{document}

\section{A Graph-View of Bilinear Structure}
\label{appendix_graph}

As mentioned above, the modeling of dimension-wise interactions focuses more on the relations between different trajectory dimensions, which could be difficult to represent by the 2D transform.
The bilinear structure used in this manuscript learns this connection relation through the outer product, pooling, and fully connected networks.
To make it easier to understand, we further explain it from a graph view.

Given an undirected graph $\mathbf{G}(t) = (\mathbf{V}(t), \mathbf{E}(t))$ with a time variable $t$, where $\mathbf{V}(t)$ is the set of vertices, which contains all the position information of one agent at time $t$, and $\mathbf{E}(t)$ is the set of edges, which represents the connection relationships between these vertices at time $t$.
Formally,
\begin{equation}
    \begin{aligned}
        \mathbf{V}(t) &= \left\{f({r_1}_t), f({r_2}_t), ..., f({r_M}_t)\right\} \\
        &= \left\{\mathbf{f}_{1, t}, \mathbf{f}_{2, t}, ..., \mathbf{f}_{M, t}\right\},
    \end{aligned}
\end{equation}
where 
\begin{equation}
    \label{eq_appendix_embed}
    \mathbf{f}_{m, t} = f({r_m}_t) \in \mathbb{R}^d
\end{equation}
indicates an embedding function to map these vertices into the high-dimension feature space.
To establish and learn the connections between these vertices, we define the trainable adjacency matrix as:
\begin{equation}
    \mathbf{A}(t) = \begin{pmatrix}
        \mathbf{W}_{1, 1}(t) & \cdots & \mathbf{W}_{1, M}(t) \\
        \vdots & \ddots & \vdots \\
        \mathbf{W}_{M, 1}(t) & \cdots & \mathbf{W}_{M, M}(t) \\
    \end{pmatrix}.
\end{equation}
Here, each matrix $\mathbf{W}_{i, j} \in \mathbb{R}^{d \times d}$ are made trainable.
They are used to describe the relation between node $i$ and node $j$ (\IE, $\mathbf{f}_{i, t}$ and $\mathbf{f}_{j, t}$).

We converge the information on the node edges by graph convolution.
Formally,
\begin{equation}
    \label{eq_appendix_graphConv}
    \mathbf{f}'_{m, t} = \sigma \left( \mathbf{W}'_m \mbox{Flatten} \left( \sum_{j=1}^{M} \mathbf{W}_{m, j}(t) \mathbf{f}_{m, t} \otimes \mathbf{f}_{j, t} \right) \right),
\end{equation}
where $\sigma$ represents a non-linear activation, and the $\mathbf{W}_m'$ is another trainable weight matrix.
Finally, we have the refined vertices
\begin{equation}
    \mathbf{V}'(t) = \left\{\mathbf{f}'_{1, t}, \mathbf{f}'_{2, t}, ..., \mathbf{f}'_{M, t}\right\}.
\end{equation}

It is worth noting that the above \EQUA{eq_appendix_graphConv} and the bilinear structure introduced in the manuscript describe the same network structure, despite their difference in representation.
To reduce unnecessary misunderstandings, we do not describe the network inference process through this graph form in the manuscript, although the use of a graph may make it easier to understand the motivation for using the bilinear model.
In addition, all the operations above are performed on time series.
If we use trajectory spectrums to replace the \EQUA{eq_appendix_embed}, and take the frequency variable $n$ to instead the time variable $t$, we have
\begin{equation}
    \mathbf{\mathcal{V}}(n) = \{\mathbf{f}_{m, n}\}_{m=1}^{\mathcal{M}},\quad\mbox{where}~\mathbf{f}_{m, n} = f(s_{n, m}).
\end{equation}
Accordingly, we have the refined vertices' spectrum representations:
\begin{equation}
    \mathbf{\mathcal{V}}'(t) = \left\{\mathbf{f}'_{1, n}, \mathbf{f}'_{2, n}, ..., \mathbf{f}'_{\mathcal{M}, n}\right\}.
\end{equation}
Then, the outer product matrix $\mathbf{R}[n, :, :]$ has become the adjacency matrix of the graph $\mathbf{G}(n) = (\mathbf{\mathcal{V}}(n), \mathbf{\mathcal{E}}(n))$ on the frequency node $n \in [1, \mathcal{N}_h]$.

It is worth noting that the methods proposed in the manuscript do not really use graph structures and graph convolution operations.
The analyses using the graph views are only intended to make it easier to understand the motivation and the rough working of bilinear structures.
Therefore, this part of the analysis is for reference only.

\end{document}
