# Supplementary material for: Another Vertical View: A Hierarchical Network for Heterogeneous Trajectory Prediction via Spectrums
Source: arXiv:2304.05106 source file (2024-12-03)
Supplement: Supplementary file 2 [file s5_skeleton.tex]

%%%%%%%%%%%%%%%%%%%%%%%
%% Author: Conghao Wong
%% Date: 2023-04-26 14:39:16
%% LastEditors: Beihao Xia
%% LastEditTime: 2023-07-04 16:37:54
%% Description: file content
%% Github: https://cocoon2wong.github.io
%% Copyright 2023 Conghao Wong, All Rights Reserved.
%%%%%%%%%%%%%%%%%%%%%%%

\documentclass[../../paper.tex]{subfiles}

\begin{document}

\section{Evolution of Motion (Skeleton) Prediction}
\label{appendix_skeleton}

\begin{table}[tbp]
    \centering
    \caption{
        Comparisons of 3D skeleton prediction performance on Human3.6M.
        Reported metrics are the FDE during different prediction periods (length of these periods are shown in milliseconds).
    }
    \label{tab_appendix_fde}
    \begin{tabular}{c|c|cccc}
        \toprule
        \multirow{2}{*}{Models} & \multirow{2}{*}{Source} & \multicolumn{4}{c}{FDE @ $t$ $\downarrow$} \\
        & & $t=$ 80 & 160 & 320 & 400 \\

        \midrule
        Res. sup.\cite{martinez2017human} & \CVPR~2017 & 34.7 & 62.0 & 101.1 & 115.5 \\
        Traj-GCN \cite{mao2019learning} & \ICCV~2019 & 26.1 & 52.3 & 63.5 & 63.5 \\
        DMGNN \cite{li2020dynamic} & \CVPR~2020 & 33.6 & 65.9 & 79.7 & 79.7 \\
        MSR-GCN \cite{dang2021msr} & \ICCV~2021 & 12.1 & 25.6 & 51.6 & 62.9 \\
        PGBIG \cite{ma2022progressively} & \CVPR~2022 & 10.3 & 22.7 & 47.4 & 58.5 \\
        SPGSN \cite{li2022skeleton} & \ECCV~2022 & 10.4 & 22.3 & 47.1 & 58.3 \\
        EqMotion \cite{xu2023eqmotion} & \CVPR~2023 & \MARK{9.1} & \MARK{20.1} & \MARK{43.7} & \MARK{55.0} \\

        \midrule
        \MODEL-Haar & (Ours) & 16.8 & 32.8 & 63.2 & 78.4 \\
        \EMODEL-Haar & (Ours) & 13.0 & 25.5 & 50.1 & 62.8 \\

        \bottomrule
    \end{tabular}

\end{table}

\begin{figure*}[tb]
    \centering
    \includegraphics[width=1.0\linewidth]{../../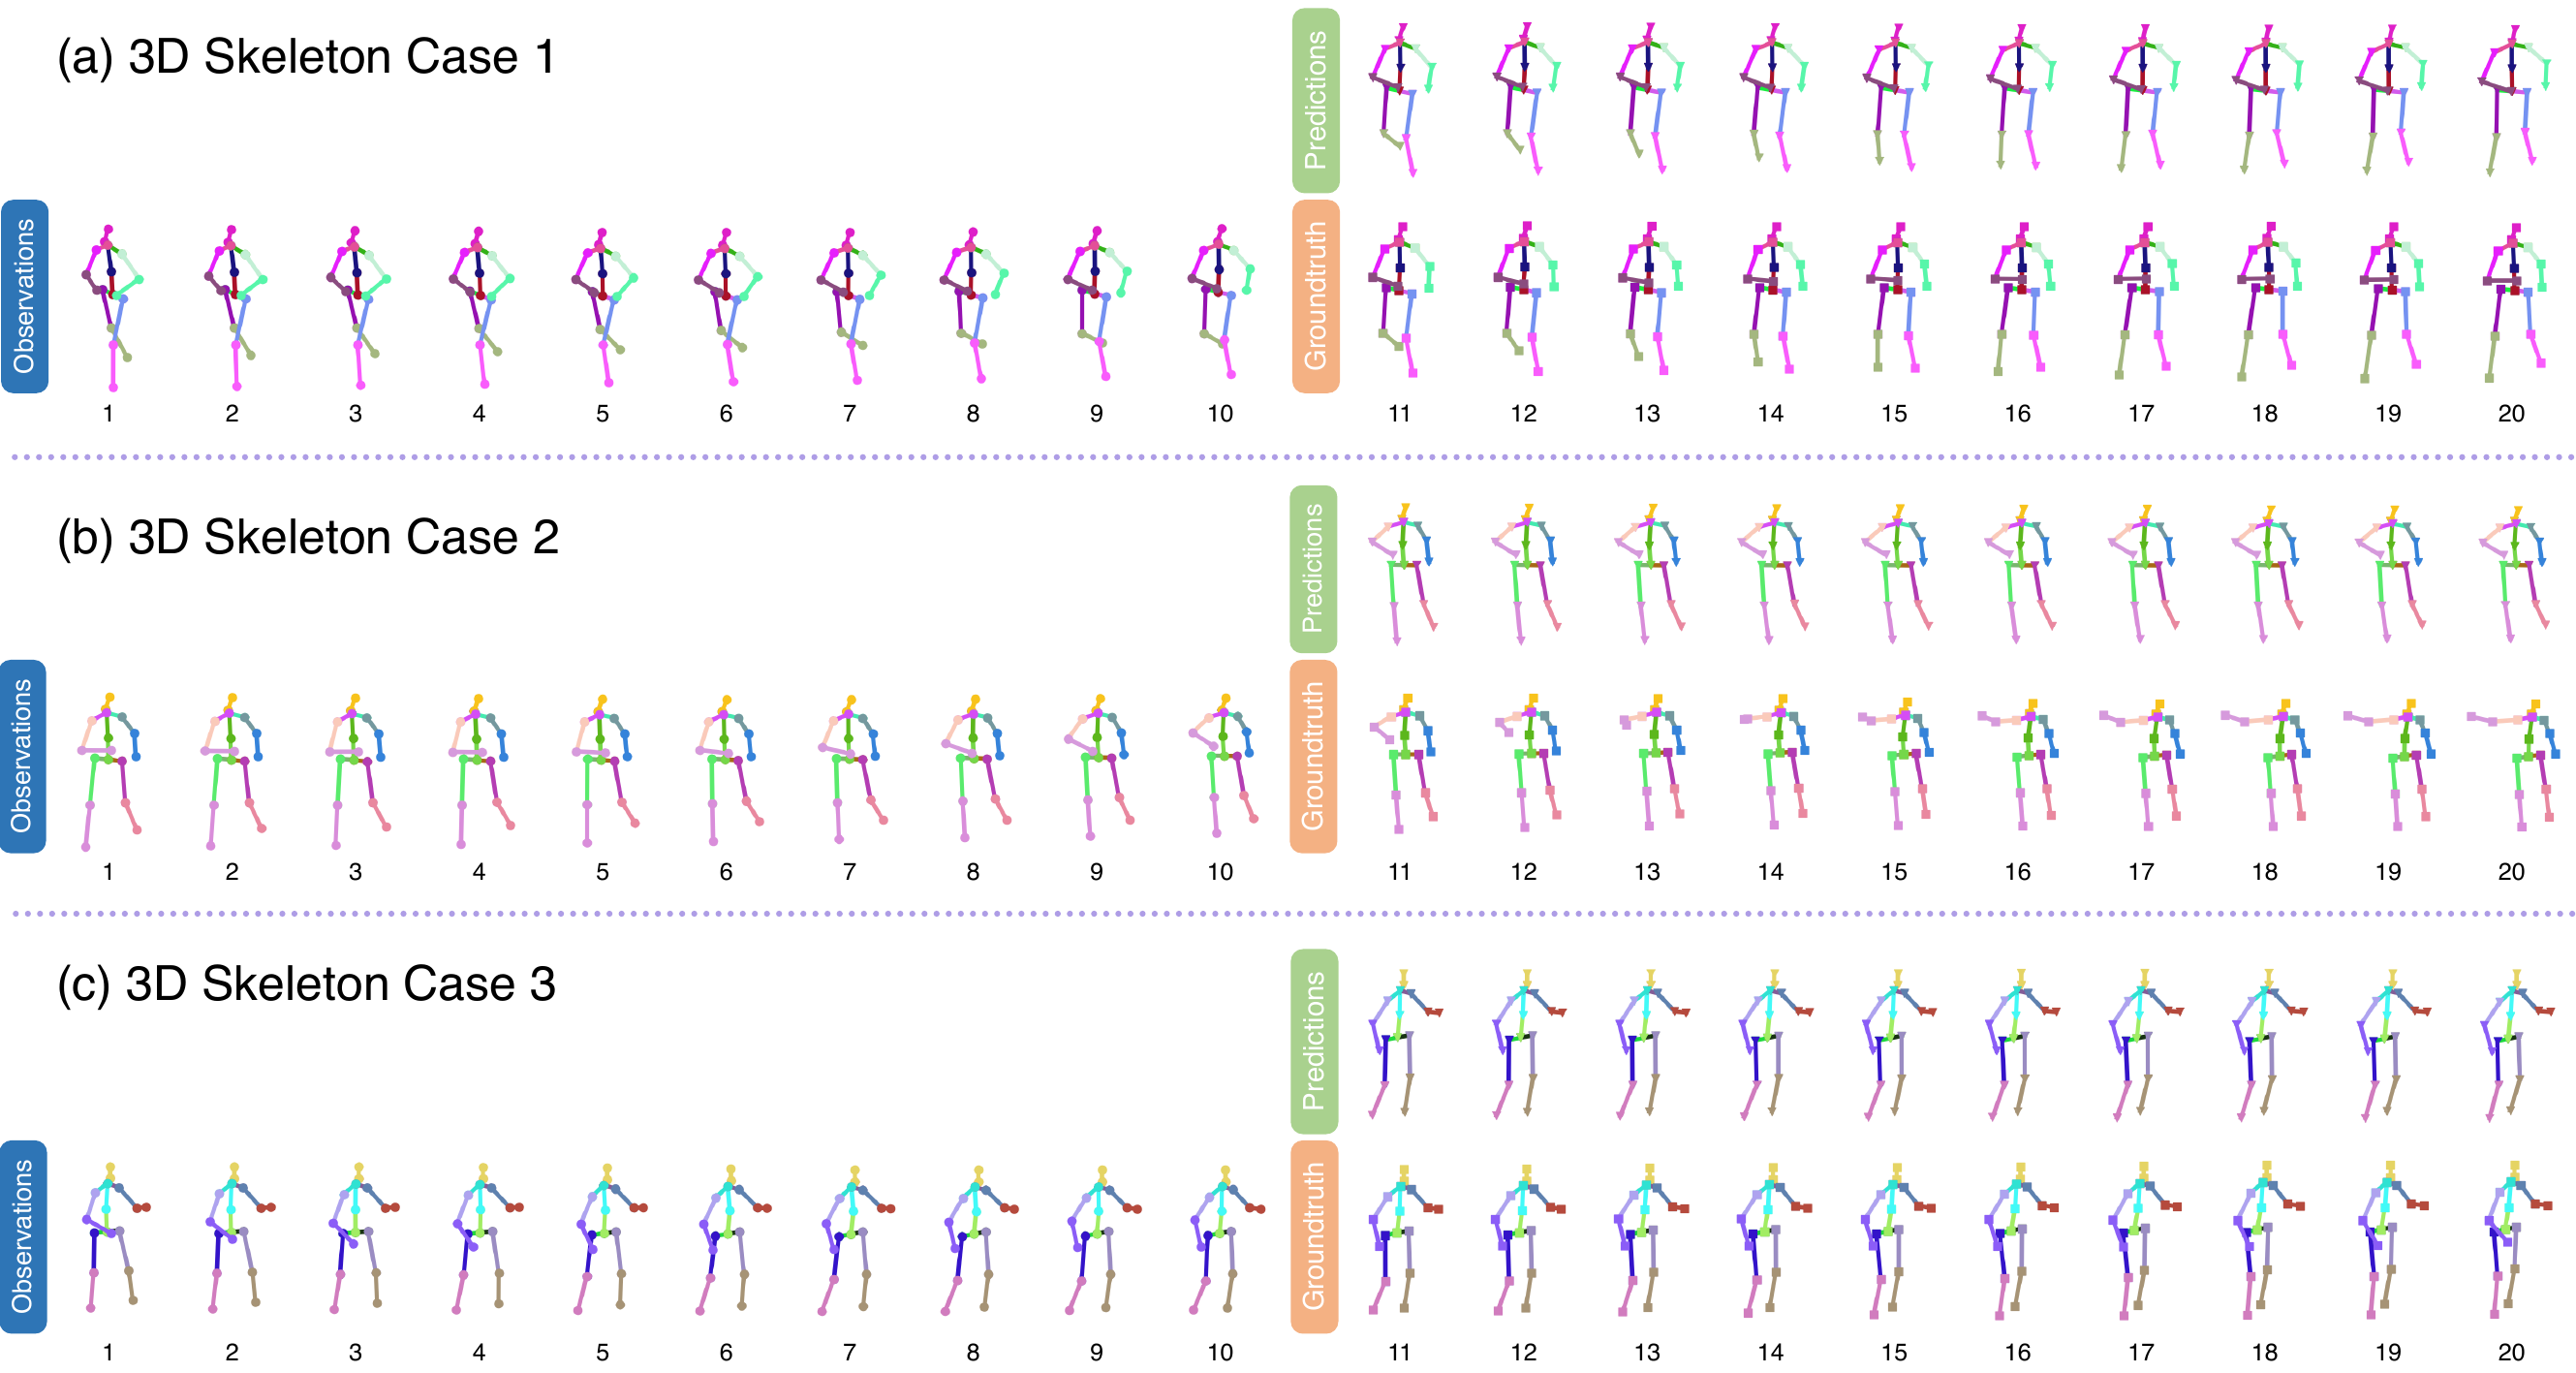}
    \caption{
        Visualized 3D skeletons predictions (3D skeleton-17) on Human3.6M.
    }
    \label{fig_appendix_skeleton}
\end{figure*}

The \EMODEL~is proposed to handle both the frequency response of trajectories and dimension-wise interactions with heterogeneous trajectories.
We have validated the proposed models with three different forms of trajectories, including \textbf{2D coordinates} ($M=2$), \textbf{2D bounding boxes} ($M=4$), and \textbf{3D bounding boxes} ($M=6$).
In order to verify more directly the modeling and prediction capabilities of the proposed model for heterogeneous trajectories, we validate the prediction performance for 3D human skeletons in this section.
The skeletons we used for validation consist of 17 3D points, which we call \textbf{3D skeleton-17} ($M=51$).
It should be noted that the proposed models (\MODEL~and \EMODEL) are not specifically designed for motion (skeleton) prediction.
We just want to verify our idea under a new type of heterogeneous trajectories.

~\\\textbf{Datasets.}
Following recent motion prediction approaches like \cite{xu2023eqmotion}, we choose the \textbf{Human3.6M}\cite{ionescu2013human3,ionescu2011latent} dataset to validate the motion prediction performance.
It is a large-scale dataset with 3.6 million 3D human poses and corresponding images, performed by 11 professional actors in 15 scenarios (such as discussion, smoking, taking photos, and talking on the phone).
Its videos and pose data are recorded at 50Hz.

~\\\textbf{Baselines.}
We choose the following methods as baselines to validate \EMODEL's skeleton prediction performance, including
Res. sup.\cite{martinez2017human},
Traj-GCN \cite{mao2019learning},
DMGNN \cite{li2020dynamic},
MSR-GCN \cite{dang2021msr},
PGBIG \cite{ma2022progressively},
SPGSN \cite{li2022skeleton},
EqMotion \cite{xu2023eqmotion}.

~\\\textbf{Metrics.}
We use the FDE (Final Displacement Error) as the metric to measure the 3D skeleton prediction performance.
It should be noted that in the field of motion prediction, this metric is also more commonly known as the Mean Per Joint Position Error (MPJPE).
For easier understanding, we still use the FDE as usual for trajectory prediction.

~\\\textbf{Implementation Details.}
Following previous settings, we use all data from subjects $\{1, 6, 7, 8, 9\}$ to train the model, subjects $\{11\}$ to validate, and subjects $\{5\}$ to test.
When making the training samples, we sample observations with the frequency of 25Hz (\IE, the sample interval is 40ms) and use $t_h = 10$ frames (400ms) of observations from all subjects to predict their possible trajectories (3D skeleton-17) for the next $t_f = 10$ frames (400ms).

We set $N_{key} = 4$, and $\{t^{key}_1, t^{key}_2, t^{key}_3, t^{key}_4\} = \{t_h + 1, t_h + 4, t_h + 7,t_h + 10\}$.
The input dimension of the network is set to $M = 17*3 = 51$.
We extend the feature dimension from 128 to 512 for each layer in the network to expand the model capacity.
We disable the noise sampling layers so that the network could predict the deterministic predictions.
In addition, since there is only one subject in the scene, all social interaction and scene interaction modules are also disabled.
When training on Human3.6M, we set the learning rate to 0.0005 and train the model for 200 epochs.

~\\\textbf{Quantitative analysis.}
We show the comparisons of the proposed \EMODEL-Haar and several state-of-the-art motion prediction baselines in \TABLE{tab_appendix_fde}.
The proposed model and MSR-GCN have similar motion prediction performance.
Although the proposed \EMODEL~does not outperform the recently proposed methods like EqMotion (for about 14.2\% performance drop), it still shows a strong competitive performance.
In addition, \EMODEL~has about 19.9\% performance gain compared to the basic \MODEL.
Both models were trained and tested under the same experimental conditions, and the only difference is that a bilinear structure is included in \EMODEL.
This comparison also quantifies the effectiveness of the proposed bilinear structure in establishing dimension-wise interactions in complex heterogeneous trajectories (3D human skeletons).

~\\\textbf{Qualitative Analysis.}
We show the visualized 3D skeleton prediction results in \FIG{fig_appendix_skeleton} to demonstrate how the proposed model handles the complex dimension-wise interactions within the trajectory.
Naturally, dimension-wise interactions in a skeleton manifest as changes and interactions of edges between different joints, and are limited by the physical constraints and motions of the human body.
The proposed model, although not purposely designed for motion prediction, still exhibits amazing prediction results.
As shown in \FIG{fig_appendix_skeleton} (a), \EMODEL~successfully predicted the subsequent movements of the person who was running.
It is particularly noteworthy that it has a better prediction of the legs in the skeleton, which is also shown in \FIG{fig_appendix_skeleton} (b) and (c).
Unfortunately, the model does not predict human arms very well.
As shown in \FIG{fig_appendix_skeleton} (c), they remain almost stationary without any motion.

~\\\textbf{Summary.}
The prediction results in the more complex human 3D skeletons ($M=51$) also demonstrate the effectiveness of the proposed \EMODEL~in dealing with dimension-wise interaction in more complex heterogeneous trajectories.
It also shows the higher trajectory prediction potential of the model without changing the model structure, which further demonstrates the generality of the proposed model ``from another view''.
However, it is worth noting that motion prediction is currently a challenging task, which is also more different from human trajectory prediction in terms of concerns and applications.
While comparisons across tasks may be inappropriate, we only try to validate the model's ability to handle dimension-wise interactions.

\end{document}
