# Supplementary material for: Another Vertical View: A Hierarchical Network for Heterogeneous Trajectory Prediction via Spectrums
Source: arXiv:2304.05106 source file (2024-12-03)
Supplement: Supplementary file 3 [file _fig_s5_skeleton.tex]

%%%%%%%%%%%%%%%%%%%%%%%
%% Author: Conghao Wong
%% Date: 2023-03-20 09:26:50
%% LastEditors: Conghao Wong
%% LastEditTime: 2023-05-04 09:27:17
%% Description: file content
%% Github: https://cocoon2wong.github.io
%% Copyright 2023 Conghao Wong, All Rights Reserved.
%%%%%%%%%%%%%%%%%%%%%%%

\documentclass[../../paper.tex]{subfiles}

\begin{document}

\begin{figure*}[tb]
    \centering
    \includegraphics[width=1.0\linewidth]{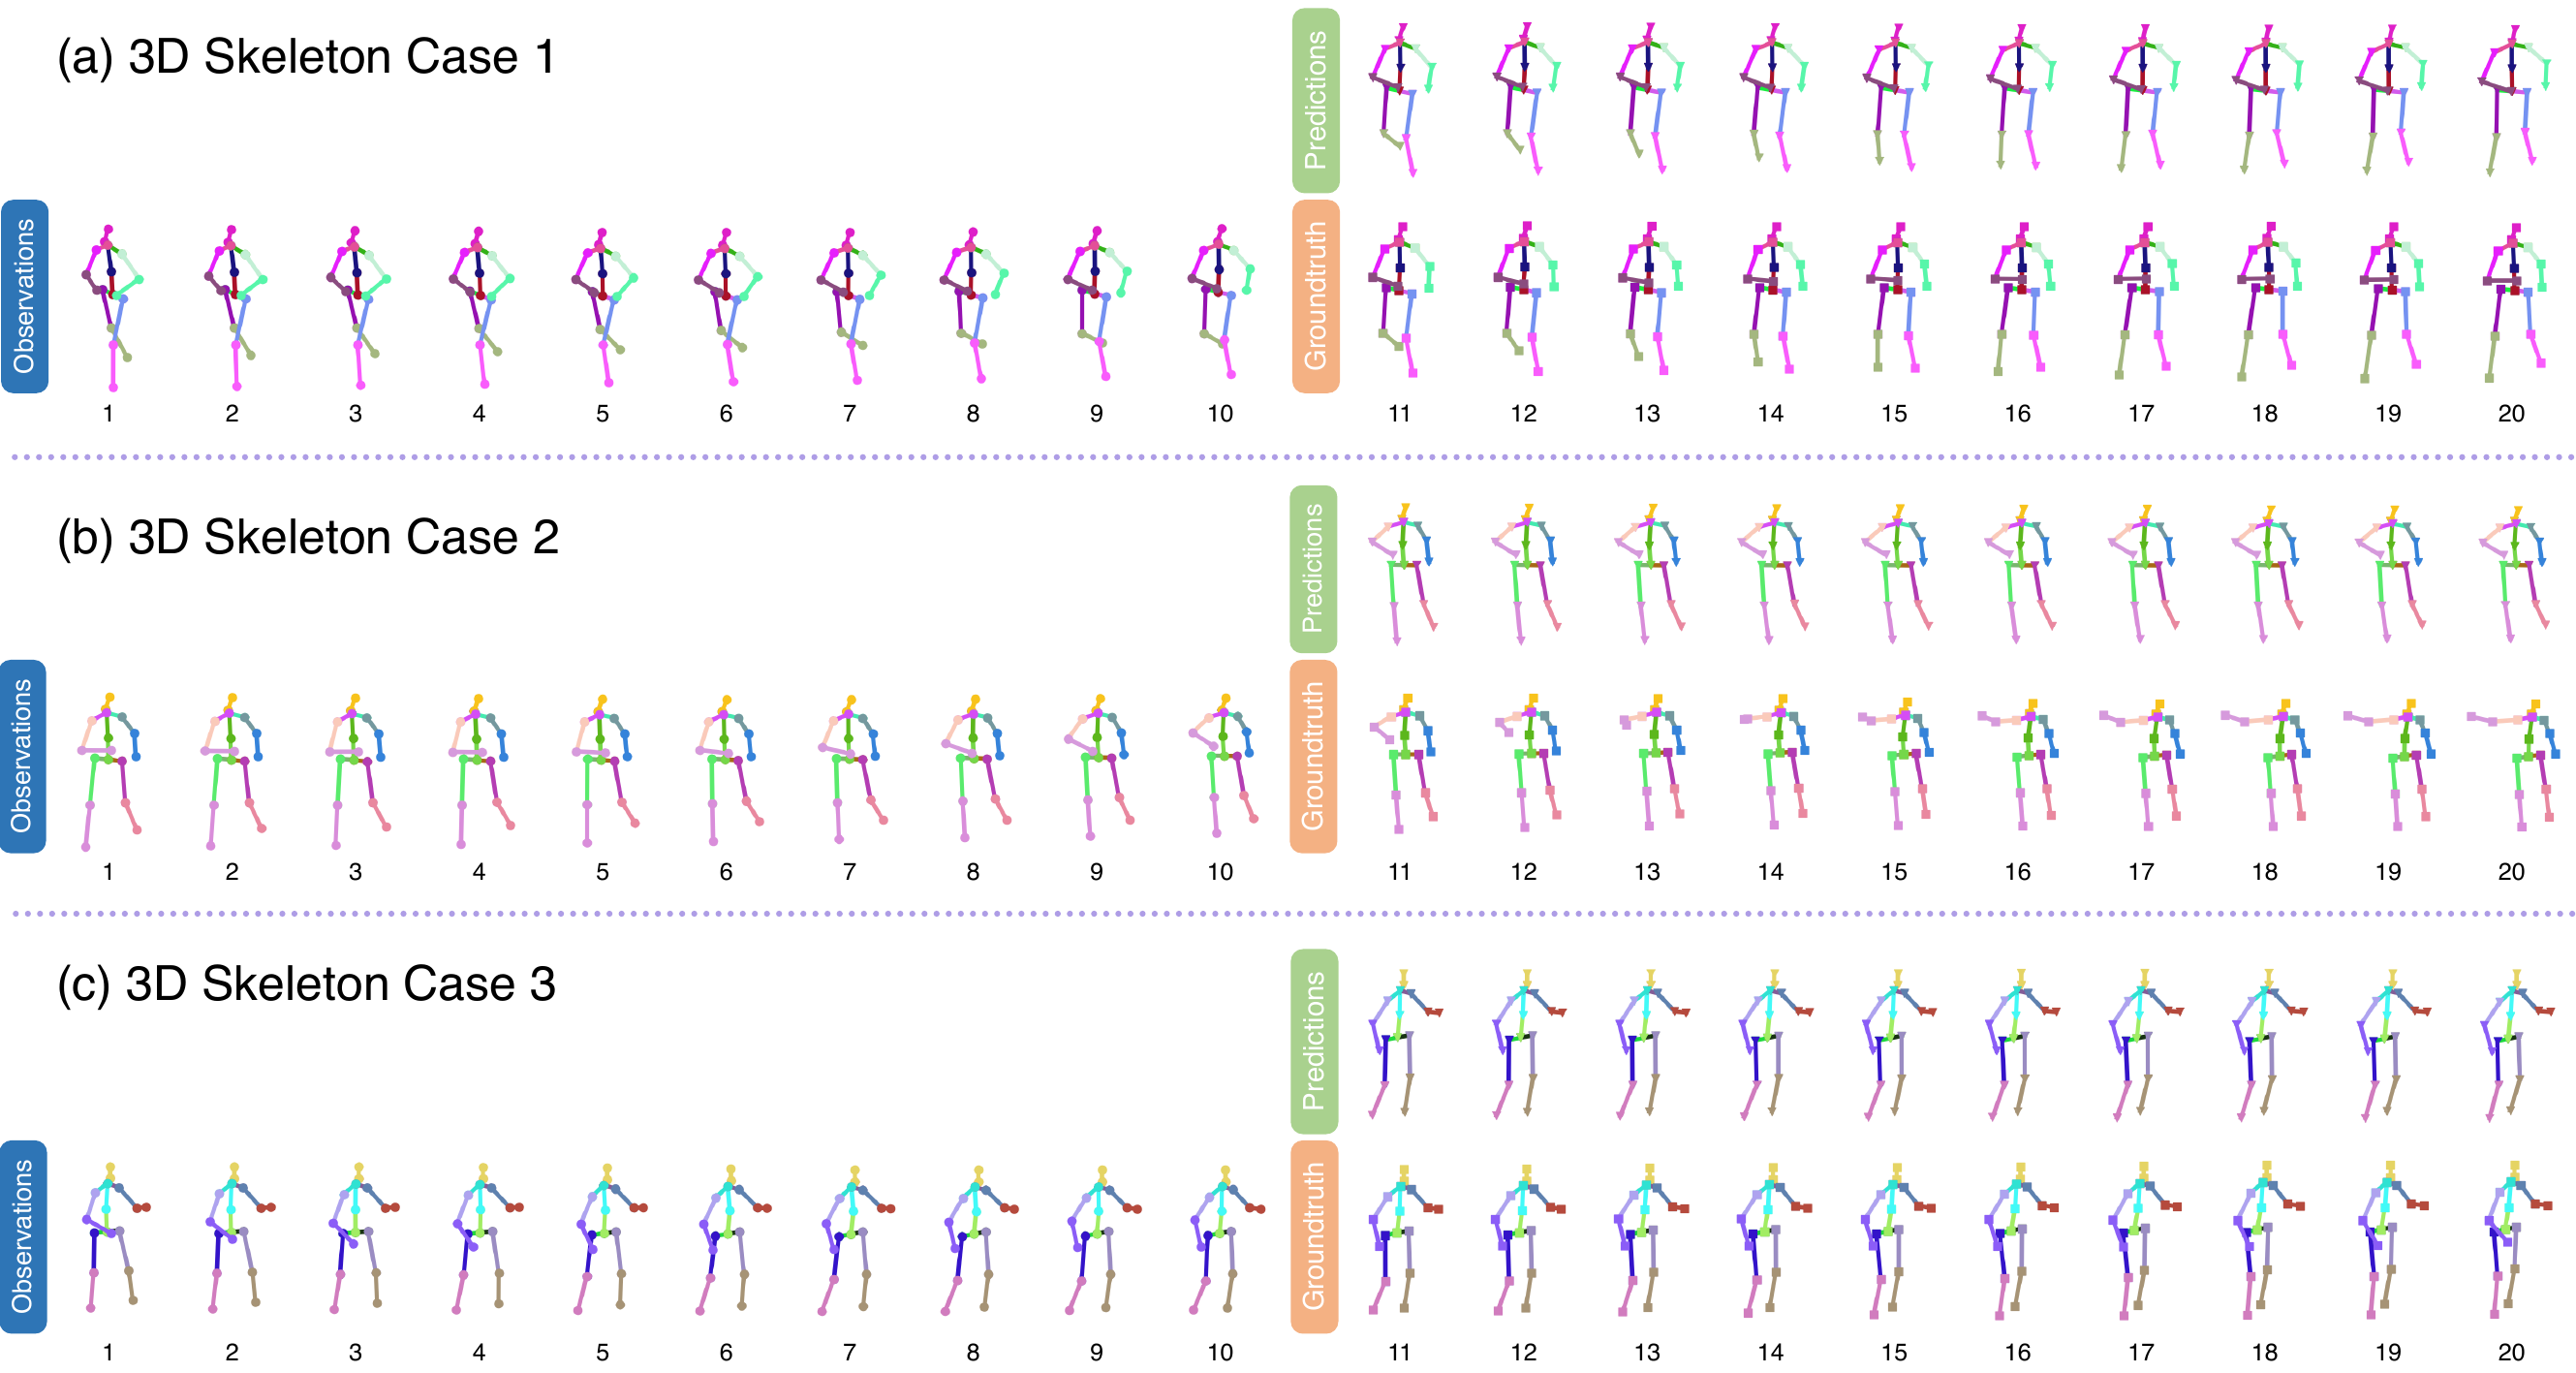}
    \caption{
        Visualized 3D skeletons predictions (3D skeleton-17) on Human3.6M.
    }
    \label{fig_appendix_skeleton}
\end{figure*}

\end{document}
