# Supplementary material for: Another Vertical View: A Hierarchical Network for Heterogeneous Trajectory Prediction via Spectrums
Source: arXiv:2304.05106 source file (2024-12-03)
Supplement: Supplementary file 4 [file _tab_s5_fde.tex]

%%%%%%%%%%%%%%%%%%%%%%%
%% Author: Conghao Wong
%% Date: 2022-12-06 09:38:43
%% LastEditors: Beihao Xia
%% LastEditTime: 2023-05-18 15:05:11
%% Description: file content
%% Github: https://github.com/cocoon2wong
%% Copyright 2022 Conghao Wong, All Rights Reserved.
%%%%%%%%%%%%%%%%%%%%%%%

\documentclass[../../paper.tex]{subfiles}

\begin{document}
    
\begin{table}[tbp]
    \centering
    \caption{
        Comparisons of 3D skeleton prediction performance on Human3.6M.
        Reported metrics are the FDE during different prediction periods (length of these periods are shown in milliseconds).
    }
    \label{tab_appendix_fde}
    \begin{tabular}{c|c|cccc}
        \toprule
        \multirow{2}{*}{Models} & \multirow{2}{*}{Source} & \multicolumn{4}{c}{FDE @ $t$ $\downarrow$} \\
        & & $t=$ 80 & 160 & 320 & 400 \\

        \midrule
        Res. sup.\cite{martinez2017human} & \CVPR~2017 & 34.7 & 62.0 & 101.1 & 115.5 \\
        Traj-GCN \cite{mao2019learning} & \ICCV~2019 & 26.1 & 52.3 & 63.5 & 63.5 \\
        DMGNN \cite{li2020dynamic} & \CVPR~2020 & 33.6 & 65.9 & 79.7 & 79.7 \\
        MSR-GCN \cite{dang2021msr} & \ICCV~2021 & 12.1 & 25.6 & 51.6 & 62.9 \\
        PGBIG \cite{ma2022progressively} & \CVPR~2022 & 10.3 & 22.7 & 47.4 & 58.5 \\
        SPGSN \cite{li2022skeleton} & \ECCV~2022 & 10.4 & 22.3 & 47.1 & 58.3 \\
        EqMotion \cite{xu2023eqmotion} & \CVPR~2023 & \MARK{9.1} & \MARK{20.1} & \MARK{43.7} & \MARK{55.0} \\

        \midrule
        \MODEL-Haar & (Ours) & 16.8 & 32.8 & 63.2 & 78.4 \\
        \EMODEL-Haar & (Ours) & 13.0 & 25.5 & 50.1 & 62.8 \\

        \bottomrule
    \end{tabular}

\end{table}

\end{document}
