# Supplementary material for: Another Vertical View: A Hierarchical Network for Heterogeneous Trajectory Prediction via Spectrums
Source: arXiv:2304.05106 source file (2024-12-03)
Supplement: Supplementary file 5 [file main.tex]

%%%%%%%%%%%%%%%%%%%%%%%
%% Author: Conghao Wong
%% Date: 2022-12-06 19:30:00
%% LastEditors: Beihao Xia
%% LastEditTime: 2024-08-21 09:34:35
%% Description: file content
%% Github: https://github.com/cocoon2wong
%% Copyright 2022 Conghao Wong, All Rights Reserved.
%%%%%%%%%%%%%%%%%%%%%%%

\documentclass[../../paper.tex]{subfiles}

\begin{document}

% \appendices

\title{
    % View Vertically: A Hierarchical Network for Trajectory Prediction via Fourier Spectrums
    Supplemental Materials for ``Another Vertical View: A Hierarchical Network for Heterogeneous Trajectory Prediction via Spectrums''
}
\maketitle

\subfile{./s6_transform.tex}
\subfile{./s1_TransformerDetails.tex}
\subfile{./s2_LinearLeastSquareForTrajectoryPrediction.tex}
\subfile{./s3_2DDFTvsBS.tex}
% \subfile{./s4_AGraphView.tex}
% \subfile{./s5_skeleton.tex}
\subfile{./s7_generalization.tex}

\bibliographystyle{IEEEtran}
\bibliography{/Users/Shared/paper/ref.bib}

\end{document}
